# Supplementary material for: Translation and Fusion Improves Zero-shot Cross-lingual Information Extraction
Source: arXiv:2305.13582 source file (2024-06-20)
Supplement: Supplementary file 1 [file appendix.tex]

\clearpage
\onecolumn

\addcontentsline{toc}{section}{Appendix}

\part{Appendix}
\parttoc

\section{Evaluation Methods}

\subsection{Evaluating Correctness}
\label{sec:grading}

For a given question with known and generated answers $(Q, A, \hat{A})$ the correctness $C$ is True if the generated answer $\hat{A}$ matches the ground truth answer $A$. 
For multiple-choice question-answering, the matching process only involves checking the first token generated via greedy decoding.  %\\

For open-ended evaluations, determining if the answer given is correct is more complex. One simple approach is to check if the ground truth answer $A$ appears as a substring of answer $\hat{A}$. However, this does not capture rephrasings that may be essentially equivalent - such as "NYC" for "New York City," or "Daoism" and "Taoism." Conversely, it also has the potential to be over-generous if the model is particularly verbose and emits many incorrect answers along with the correct string. 
Given the difficulty involved in writing a rule-based method for evaluating open-ended answer correctness, we use instead a strong auxiliary language model to evaluate correctness. The auxiliary language model is shown the query $Q$, the ground truth answer $A$, and the model's output $\hat{A}$, and is prompted to grade the answer whilst tolerating nuance. For full details of the prompt used see (\cref{fig:prompts}). In this paper we utilise GPT 3.5 Turbo as the auxiliary grading model.
We conduct a comparison of human grading, substring grading, and GPT 3.5 Turbo grading on select subsets of MMLU in \cref{app:oe-grading}. We find that humans and GPT 3.5 Turbo have much greater agreement than humans and the substring method.

\subsection{Grading}
\label{app:grading-prompt}

\paragraph{Dataset Construction.}
To perform calibration-tuning ({\sc CT}), we need tuples $(Q, A, \hat{A}, C)$, answers from a language model that have been graded for correctness. When calibration-tuning on multiple choice questions, we can use an exact string match to generate $C$. To grade open-ended answers, we use a strong language model and \emph{grading prompt} $G$ instead (\cref{fig:prompts}):
\begin{itemize}[topsep=0pt]
    \setlength\itemsep{0em}
    \item $\boldsymbol{G}$: a prompt used for grading answers $\boldsymbol{\hat{A}}$ with $\boldsymbol{A}$.
\end{itemize}
Compared to alternatives like exact match, language model grading is insensitive to re-phrasings that are equivalent in meaning - such as ``NYC" and ``New York City," or ``Daoism" and ``Taoism". 
LLM grading can also penalize answers that are overly verbose or use a different meaning of the same word, potentially containing incorrect answers along with the correct string. 
For example, if the question is ``What's it called when you move quickly by foot and both feet aren't always touching the ground?'' and the LLM response is ``A bank run", the grader should be able to distinguish that this is semantically dissimilar to the true answer ``run''. 

In this paper, we utilize GPT 3.5 Turbo as the auxiliary grading model. When comparing many possible grading methods on subsets of MMLU, we find that GPT 3.5 Turbo has high agreement with humans while being cost efficient (\cref{app:oe-grading}).

\begin{figure}[!ht]
    \centering

\begin{adjustbox}{width=0.5\linewidth}
    
    \begin{tabular}{|p{0.5\linewidth}|}
    \toprule

    \textbf{Grading prompt} $(\boldsymbol{G})$\\
    \midrule
    
    {    
    The problem is: $\boldsymbol{Q}$ \newline
    The correct answer is: $\boldsymbol{A}$ \newline
    A student submitted: $\boldsymbol{\hat{A}}$ \newline
    \newline
The student's answer must be correct and specific but not overcomplete (for example, if they provide two different answers, they did not get the question right). However, small differences in formatting should not be penalized (for example, `New York City' is equivalent to `NYC'). Did the student provide an equivalent answer to the ground truth? Please answer yes or no without any explanation: $\boldsymbol{C}$ \texttt{</s>}
    }
    
    \\
    \bottomrule
    \end{tabular}
\end{adjustbox}    
    \caption{For open-ended generation, we calculate the ground-truth correctness $C$ using a LLM and a grading prompt ($G$). The token \texttt{</s>} is an end-of-sentence token. {\color{blue}\textbf{Blue text}} is included in the loss function when calibration-tuning.}
    \label{fig:prompts}
\end{figure}

\subsection{Comparison of Grading Techniques}
\label{app:oe-grading}

We conducted an analysis of the methods outlined in \cref{sec:grading} for open-ended evaluation. First, the base LLaMA-2 13b-chat model was prompted with questions from the following test subsets of MMLU: World Religions, Philosophy, Anatomy, High School Chemistry and Elementary School Math. The questions were stripped of their multiple-choice options before being supplied to the model.

A response was generated by the model via greedy decoding and this response was compared to the ground truth answer. The grading methods tested were Human, Substring Match, GPT 3.5 Turbo, and GPT 4.

The humans (a subset of our authors) were tasked to judge if the model response was essentially equivalent to the ground truth. For substring match, equivalence was determined by simply checking whether the ground truth answer existed as a substring within the model response. For GPT 3.5 Turbo and GPT 4, the models were supplied with the question, the ground truth, and the base model response, as well as a prompt indicating they should determine essential equivalence - see \cref{fig:prompts}.

\begin{table}[ht]
\centering
\begin{adjustbox}{width=.6\linewidth}
\begin{sc}
\begin{tabular}{l|c|c|c}
\toprule
MMLU Subset    & Substring Match & GPT3.5 & GPT4 \\ \midrule
World Religions         & 21.6\%                                  & 6.4\%                          & 1.8\%                        \\
Philosophy              & 22.8\%                                  & 2.3\%                          & 14.5\%                       \\
Anatomy                 & 13.3\%                                  & 14.8\%                         & 1.5\%                        \\
Chemistry               & 13.8\%                                  & 5.4\%                          & 1.0\%                        \\
Math                    & 12.4\%                                  & 14.8\%                         & 3.7\%                        \\
\midrule
\textbf{Average}        & \textbf{16.8\%}                         & \textbf{8.7\%}                 & \textbf{4.5\%}               \\
\bottomrule
\end{tabular}
\end{sc}
\end{adjustbox}
\vspace{2mm}
\caption{Absolute differences in accuracy \% for the different grading methods vs human estimated accuracy. A lower value corresponds to an accuracy estimate closer to the human estimate.}
\label{tab:oe-grading-diffs}
\end{table}

We recorded the binary decision on correctness for each query and response by each of the grading methods above. Taking the human scores as the gold standard of correctness, we computed the model accuracy for each subset, and then derived the absolute error in estimate of model accuracy by each of the other grading methods. These are displayed in \cref{tab:oe-grading-diffs}. We see that GPT4 is a better estimator of human-judged correctness than GPT 3.5 Turbo, which in turn is substantially better than substring match; although there is some variance on a per-subset basis. For expediency of processing time and cost, we chose to use GPT 3.5 Turbo in this paper.

\subsection{Metrics}
\label{app:ece}

\paragraph{ECE} Given $N$ samples and $B$ equally-spaced bins $b_j$, examples are assigned to bins based on the confidence of the model, and ECE is estimated as
$\widehat{\text{ECE}} = \sum_{j=1}^B \frac{\lvert b_j \rvert}{N} \left\lvert \mathrm{conf}(b_j) - \mathrm{acc}(b_j) \right\rvert$
where $\mathrm{conf}(b_j)$ is the average confidence of samples in bin $b_j$, $\mathrm{acc}(b_j)$ is the accuracy within the bin, and $\lvert b_j \rvert$ is the number of samples assigned to bin $j$. In our experiments $\mathrm{conf}$ is equivalent to $P(\text{correct})$.

\subsection{MMLU Supercategory Classifier}
\label{app:mmlu-supercategories}

To understand the impact of the subject matter of the training data on generalization, we follow the prescription of \citet{Hendrycks2020MeasuringMM} and categorize each of the 57 tasks into one of four supercategories - Humanities, STEM, Social Sciences, and Other. Since we do not have such a categorization for the training set, we must estimate their proportions.

First, we use the OpenAI embeddings (dimension 1536) of the MMLU samples with their ground truth supercategories to train a linear 4-way classifier with 10 samples from each of the 57 tasks. We use AdamW \citep{Loshchilov2017FixingWD} with learning rate 1e-3 and weight decay 1e-2. This classifier is then used to estimate the categories of each sample in the training set used for fine-tuning. Subsequently, the breakdown of results in \cref{fig:mmlu_transfer} (Left) follows.

\section{Baseline Methods}

\subsection{Sampling Methods}
\label{app:sampling-baselines}

We use two baselines which obtain an estimate of certainty by sampling the same answers $n=10$ times and then estimating the proportion of sampled answers that agree with the greedily decoded ``main" answer. There are several critical downsides to these approaches: (i) the uncertainty here depends on the sampling parameters---for example, in the limit where the sampling converges to mere greedy decoding, the LLM will produce $n$ identical samples, and therefore the certainty will always be 1---(ii) these approaches require $O(n)$ answer generations to provide a certainty estimate for a single generation. The intense computational restriction prevents us from easily searching the space of sampling parameters for the optimal set, so we choose parameters arbitrarily; here we sample with top$\_p = 0.95$.

\paragraph{Counting} In this baseline, each sampled answer is compared to the greedy answer by prompting an expert LLM with both answers and asking it to judge their equivalence. The proportion of samples that are equivalent to the greedy answer is the certainty estimate. This baseline is similar to \emph{Label prob} \cite{tian2023just}; our method differs by not choosing the argmax semantic group as the final prediction, but instead using the greedy decode for the final prediction, so as to maintain the same accuracy performance as our uncertainty query method. This met

\paragraph{Likelihood accumulation} In this baseline, we add up likelihoods of sampled answers to estimate the mass associated with the predicted answer. We begin by prompting an expert LLM in order to find which sampled answers are equivalent to the greedy answer---like in the counting baseline. In this method, the certainty estimate is produced by adding the length-normalized likelihoods of those sampled answers equivalent to the greedy answer, and dividing this quantity by the sum of all sampled answers' length-normalized likelihoods. This procedure of adding likelihoods of samples in order to estimate the likelihood of an equivalence class is similar to that used by \cite{Kuhn2023SemanticUL}, although they do not use it for certainty estimates but instead to produce entropy scores. In practice, the scores produced by these two methods are actually very similar---so we report only likelihood accumulation numbers in the main text.

\subsection{Verbal Elicitation}
\label{app:ve-baseline}

Although \citet{tian2023just} introduce several strategies for prompting, involving multiple guesses or multiple stages of interleaving prompting and generation, we did not find that any strategy consistently outperformed any other. This finding was consistent with the results of \citet{Xiong2023CanLE}. Ultimately, for convenience, we adopted a two stage strategy with a single guess because it can be used in tandem with logged datasets of generated answers per model.

The exact prompt we used is essentially the same at in \citep{tian2023just}, but with small modifications that improved the rate of correctly formatted responses:

\begin{quote}
``Provide the probability that your answer is correct. Give ONLY the probability, no other words or explanation.

For example:

Probability: <the probability between 0.0 and 1.0 that your guess is correct, without any extra commentary whatsoever; just the probability!>

Include probability for the answer below:
Probability:''
\end{quote}

Verbal elicitation methods typically output complex strings containing both answers and associated probabilities. This means that if any element of parsing fails, it can be challenging to construct partial results. This effect tends to diminish when using large models, which are more responsive to zero-shot prompting.

\paragraph{Parsing Details}
The original verbal elicitation prompts are given in the appendix of  \citep{tian2023just}. However, it is not clear how the original authors decide to parse answers from the generations and how failure to parse is handled. When we fail to parse the guess from the generation we return an empty string and associated probability 0.5. When we fail to parse a probability, we also return probability 0.5. For versions with multiple guesses, if any part of the parsing processes fails in an ambiguous way, we default back to an empty string for the answer and 0.5 for the probability. The only unambiguous cases are those which explicit succeed in the generating a valid guess and probability in the first case but not subsequent cases. In this scenario, we default to using the successfully parse first guess and associated probability.

\section{Fine-tuning Method}

\subsection{Regularization Term}
\label{app:regularization}

To keep the calibration-tuned parameters $\theta$ within the neighborhood of the initial parameters, $\theta_0$, we use a regularization term that penalizes the divergence between the original sampling distribution and the calibration-tuned model on the target sequence $A$, yielding regularization $\mathcal{R}(\theta; \theta_0)$, which we use with weighting parameter $\kappa$.

Specifically, let $p_{\theta_0}$ be the language modeling distribution of the language model we wish to calibration-tune, and $q_\theta$ be the corresponding language modeling distribution as a consequence of calibration-tuning.
We then use the Jensen-Shannon Divergence ${\mathrm{JSD}(p_{\theta_0} \parallel q_\theta)}$ \citep{MacKay2004InformationTI} between the two language modeling distributions as the regularizer, where ${\mathrm{JSD}(p \parallel q) \defeq \nicefrac{1}{2}(\kl(p \parallel m) + \kl(q \parallel m))}$, where $m \defeq \nicefrac{1}{2}(p + q)$ is the mixture distribution.
JSD regularization is applied only to the logits corresponding to the target sequence $A$.

We note that using either direction of KL-divergence, i.e. the forward-KL $\mathrm{KL}(p_{\theta_0} \parallel q_{_\theta})$ or reverse-KL $\mathrm{KL}(q_{_\theta} \parallel p_{\theta_0})$ was insufficient for optimal performance with calibration tuning. 
The forward KL-divergence encourages a zero-avoiding behavior such that the mass of $q_\theta$ is spread across multiple modes of $p_{\theta_0}$ to minimize the KL-divergence to avoid assigning no mass to regions of the probability space.
To the contrary, the reverse KL-divergence encourages a zero-forcing behavior such the $q_\theta$ only needs to cover any one mode of $p_{\theta_0}$ \citep{bishop2006pattern}.
It is not necessarily obvious which one of these behaviors one should prefer for the specific case of large language models. Therefore, as a practical choice, we pick the one that provides us the most performant calibration-tuned model. 

\subsection{Training Data}
\label{app:training-data}

We reserve the following datasets for training.

\begin{itemize}[itemsep=0ex,topsep=0pt]
\item AI2 Reasoning Challenge (ARC) \citep{Clark2018ThinkYH}, 
\item Boolean Questions (BoolQ) \citep{Clark2019BoolQET}, 
\item CommonsenseQA \citep{Talmor2019CommonsenseQAAQ}, 
\item CosmosQA \citep{Huang2019CosmosQM}, 
\item HellaSwag \citep{Zellers2019HellaSwagCA}, 
\item MathQA \citep{amini-etal-2019-mathqa}, 
\item Recognizing Textual Entailment (RTE/SNLI) \citep{Bowman2015ALA},
\item Adversarial NLI \citep{Nie2019AdversarialNA}, 
\item OpenBookQA \citep{Mihaylov2018CanAS}, 
\item PIQA \citep{Bisk2019PIQARA}, 
\item SciQ \citep{Welbl2017CrowdsourcingMC}, 
\item The CommitmentBank (CB) \citep{de2019commitmentbank}, 
\item Multi-Sentence Reading Comprehension (MultiRC) \citep{Khashabi2018LookingBT}, 
\item Choice of Plausible Alternatives (CoPA) \citep{Gordon2011SemEval2012T7}, 
\item TREC \citep{Li2002LearningQC}, 
\item Adversarial Winograd (Winogrande) \citep{Sakaguchi2019WINOGRANDEAA}.
\end{itemize}

\subsection{Training Hyperparameters}
\label{sec:mcqa-hypers}

We use HuggingFace Transformers \citep{wolf-etal-2020-transformers} and PyTorch \citep{Paszke2019PyTorchAI} for the implementation of these models. 
For all our experiments, we use the AdamW optimizer \citep{Loshchilov2017FixingWD} with a learning rate of $10^{-4}$, a cosine decay schedule, and effective batch size $M = 32$. 
The training runs for $G= 10000$ with an initial linear warmup schedule for $1000$ steps. 

\section{Extended MMLU Results}
\label{sec:mmlu_task_breakdown}

We report the breakdown of uncertainty query accuracy and ECE on all MMLU tasks in \cref{fig:mmlu_mcqa_bar1,fig:mmlu_mcqa_bar2,fig:mmlu_oe_bar1,fig:mmlu_oe_bar1,fig:mmlu_oe_bar2}.

\begin{figure*}[ht]
    \centering
    \includegraphics[width=\linewidth]{figures/mcqa_bar_plots_per_category_0.pdf}
    \caption{(Part 1) ECE and AUROC values for \texttt{Query}, \texttt{CT-Probe}, \texttt{CT-LoRA}, and \texttt{CT-Query} for each subset of MMLU in multiple-choice question answering (MCQA) setting.}
    \label{fig:mmlu_mcqa_bar1}
\end{figure*}

\begin{figure*}[ht]
    \centering
    \includegraphics[width=\linewidth]{figures/mcqa_bar_plots_per_category_1.pdf}
    \caption{(Part 2) ECE and AUROC values for \texttt{Query}, \texttt{CT-Probe}, \texttt{CT-LoRA}, and \texttt{CT-Query} for each subset of MMLU in multiple-choice question answering (MCQA) setting.}
    \label{fig:mmlu_mcqa_bar2}
\end{figure*}

\begin{figure*}[ht]
    \centering
    \includegraphics[width=\linewidth]{figures/oe_bar_plots_per_category_0.pdf}
    \caption{(Part 1) ECE and AUROC values for \texttt{Query}, \texttt{CT-Probe}, \texttt{CT-LoRA}, and \texttt{CT-Query} for each subset of MMLU in open-ended (OE) setting.}
    \label{fig:mmlu_oe_bar1}
\end{figure*}

\begin{figure*}[ht]
    \centering
    \includegraphics[width=\linewidth]{figures/oe_bar_plots_per_category_1.pdf}
    \caption{(Part 2) ECE and AUROC values for \texttt{Query}, \texttt{CT-Probe}, \texttt{CT-LoRA}, and \texttt{CT-Query} for each subset of MMLU in open-ended (OE) setting.}
    \label{fig:mmlu_oe_bar2}
\end{figure*}

\section{Confidence as a Function of Target Length}
\label{sec:conf_vs_target_len}

As we noted when motivating calibration tuning, one limitation of sequence-level probabilities is their intrinsic connection to sequence length. The probability of a sequence decreases with increasing length, regardless of the correctness of the response. By contrast, we wouldn't expect concept-level probabilities to have any discernible relationship with sequence length. In \cref{sec:conf_vs_target_len}, we show there is no consistent relationship between the confidence estimated by the calibration-tuned model and target sequence length on MMLU tasks. 

A key limitation of using token likelihoods is that they necessarily decay with the length of the generation. 
In \cref{fig:conf_vs_target_len_1,fig:conf_vs_target_len_2,fig:conf_vs_target_len_3}, we confirm over all subsets of MMLU that the length of the target does not strongly correlate with the confidence associated with the targets.
This behavior is an essential ingredient towards an effective confidence estimation in practice, such that longer sequences are not penalized in confidence despite being correct.

\begin{figure*}[!t]
    \centering
\begin{tabular}{cccc}
   \includegraphics[width=.2\linewidth]{figures/conf_vs_length/abstract_algebra.pdf} &
   \includegraphics[width=.2\linewidth]{figures/conf_vs_length/anatomy.pdf} & 
   \includegraphics[width=.2\linewidth]{figures/conf_vs_length/astronomy.pdf} & 
   \includegraphics[width=.2\linewidth]{figures/conf_vs_length/clinical_knowledge.pdf} \\ 
   \includegraphics[width=.2\linewidth]{figures/conf_vs_length/college_biology.pdf} & 
   \includegraphics[width=.2\linewidth]{figures/conf_vs_length/college_chemistry.pdf} & 
   \includegraphics[width=.2\linewidth]{figures/conf_vs_length/college_computer_science.pdf} &
   \includegraphics[width=.2\linewidth]{figures/conf_vs_length/college_mathematics.pdf} \\
   \includegraphics[width=.2\linewidth]{figures/conf_vs_length/college_medicine.pdf} & 
   \includegraphics[width=.2\linewidth]{figures/conf_vs_length/computer_security.pdf} & 
   \includegraphics[width=.2\linewidth]{figures/conf_vs_length/econometrics.pdf} & 
   \includegraphics[width=.2\linewidth]{figures/conf_vs_length/electrical_engineering.pdf} \\ 
   \includegraphics[width=.2\linewidth]{figures/conf_vs_length/elementary_mathematics.pdf} & 
   \includegraphics[width=.2\linewidth]{figures/conf_vs_length/formal_logic.pdf} & 
   \includegraphics[width=.2\linewidth]{figures/conf_vs_length/global_facts.pdf} & 
   \includegraphics[width=.2\linewidth]{figures/conf_vs_length/high_school_biology.pdf} \\ 
   \includegraphics[width=.2\linewidth]{figures/conf_vs_length/high_school_chemistry.pdf} & 
   \includegraphics[width=.2\linewidth]{figures/conf_vs_length/high_school_computer_science.pdf} & 
   \includegraphics[width=.2\linewidth]{figures/conf_vs_length/high_school_european_history.pdf} & 
   \includegraphics[width=.2\linewidth]{figures/conf_vs_length/high_school_geography.pdf} \\ 
   \includegraphics[width=.2\linewidth]{figures/conf_vs_length/high_school_government_and_politics.pdf} & 
   \includegraphics[width=.2\linewidth]{figures/conf_vs_length/high_school_macroeconomics.pdf} &
       \includegraphics[width=.2\linewidth]{figures/conf_vs_length/high_school_mathematics.pdf} &
\includegraphics[width=.2\linewidth]{figures/conf_vs_length/high_school_microeconomics.pdf}
\end{tabular}
    \caption{Confidence versus Target Length for various MMLU subsets. A horizontal regression line indicates weak correlation of confidence with the target length. See \cref{fig:conf_vs_target_len_2,fig:conf_vs_target_len_3} for other subsets.}
    \label{fig:conf_vs_target_len_1}
\end{figure*}

\begin{figure*}[!t]
    \centering
\begin{tabular}{cccc}
    \includegraphics[width=.2\linewidth]{figures/conf_vs_length/high_school_physics.pdf} &
    \includegraphics[width=.2\linewidth]{figures/conf_vs_length/high_school_psychology.pdf} & 
    \includegraphics[width=.2\linewidth]{figures/conf_vs_length/high_school_statistics.pdf} &
    \includegraphics[width=.2\linewidth]{figures/conf_vs_length/high_school_us_history.pdf} \\ 
    \includegraphics[width=.2\linewidth]{figures/conf_vs_length/high_school_world_history.pdf} &
    \includegraphics[width=.2\linewidth]{figures/conf_vs_length/human_aging.pdf} & 
    \includegraphics[width=.2\linewidth]{figures/conf_vs_length/human_sexuality.pdf} &
    \includegraphics[width=.2\linewidth]{figures/conf_vs_length/international_law.pdf} \\ 
    \includegraphics[width=.2\linewidth]{figures/conf_vs_length/jurisprudence.pdf} & 
    \includegraphics[width=.2\linewidth]{figures/conf_vs_length/logical_fallacies.pdf} & 
    \includegraphics[width=.2\linewidth]{figures/conf_vs_length/machine_learning.pdf} & 
    \includegraphics[width=.2\linewidth]{figures/conf_vs_length/management.pdf} \\
    \includegraphics[width=.2\linewidth]{figures/conf_vs_length/marketing.pdf} & 
    \includegraphics[width=.2\linewidth]{figures/conf_vs_length/medical_genetics.pdf} & 
    \includegraphics[width=.2\linewidth]{figures/conf_vs_length/miscellaneous.pdf} &
    \includegraphics[width=.2\linewidth]{figures/conf_vs_length/moral_disputes.pdf} \\ 
    \includegraphics[width=.2\linewidth]{figures/conf_vs_length/moral_scenarios.pdf} & 
    \includegraphics[width=.2\linewidth]{figures/conf_vs_length/nutrition.pdf} & 
    \includegraphics[width=.2\linewidth]{figures/conf_vs_length/philosophy.pdf} & 
    \includegraphics[width=.2\linewidth]{figures/conf_vs_length/prehistory.pdf} \\ 
    \includegraphics[width=.2\linewidth]{figures/conf_vs_length/professional_accounting.pdf} & 
    \includegraphics[width=.2\linewidth]{figures/conf_vs_length/professional_psychology.pdf} & 
    \includegraphics[width=.2\linewidth]{figures/conf_vs_length/public_relations.pdf} &
    \includegraphics[width=.2\linewidth]{figures/conf_vs_length/security_studies.pdf}
\end{tabular}
    \caption{Continuing from \cref{fig:conf_vs_target_len_1}. See also \cref{fig:conf_vs_target_len_3}.}
    \label{fig:conf_vs_target_len_2}
\end{figure*}

\begin{figure*}[!t]
    \centering
\begin{tabular}{cccc}
    \includegraphics[width=.2\linewidth]{figures/conf_vs_length/sociology.pdf} &
    \includegraphics[width=.2\linewidth]{figures/conf_vs_length/us_foreign_policy.pdf} &
        \includegraphics[width=.2\linewidth]{figures/conf_vs_length/virology.pdf} &
        \includegraphics[width=.2\linewidth]{figures/conf_vs_length/world_religions.pdf}
\end{tabular}
    \caption{Continuing from \cref{fig:conf_vs_target_len_1,fig:conf_vs_target_len_2}.}
    \label{fig:conf_vs_target_len_3}
\end{figure*}

\section{Generalization to Coding Tasks}
\label{sec:generalization-coding}

Because there are no coding tasks in our training dataset, we can use a coding competition task introduced in LiveCodeBench~\citep{jain2024livecodebench} to assess how well finetuned uncertainty estimation methods perform on completely out of distribution tasks.

To conduct the analysis in \cref{tab:coding}, we evaluate several base models on the 62 LeetCode easy questions from the livecodebench\_generation\_lite task. We asking for the model to write a Python solution and grade the solution using test cases (marking it as correct iff it passes all test cases). We then apply \texttt{Lora + Prompt} and \texttt{Zero-Shot Classifier} uncertainty estimation methods---with these methods \emph{only} using training/temperature scaling data from our main dataset mixture which notably does not include any coding tasks \cref{app:training-data}. Accuracy is shown to contextualize the model's overall level of performance on the task. On Mistral-7B, the best performing model on the coding task, the supervised \texttt{Lora + Prompt} approach dramatically improves calibration and selective prediction as compared to \texttt{Zero-Shot Classifier}; on the worse-performing Mistral-7B-Instruct and LLaMa-2-7B, selective prediction improves but calibration slightly degrades.

\begin{table}
    \centering
    \begin{tabular}{c|c|c|c|c}
    \toprule
    Model & Method & Acc & ECE & AUROC \\
    \hline
    \multirow{2}{*}{LLaMa-2-7B}	&	Zero-Shot Classifier	&	3.2\%	&	41.0\%	&	56.9\%	\\	
    	&	Lora + Prompt	&	3.2\%	&	46.4\%	&	80.0\%	\\	
    \multirow{2}{*}{Mistral-7B}	&	Zero-Shot Classifier	&	27.4\%	&	70.2\%	&	66.2\%	\\	
   	&	Lora + Prompt	&	27.4\%	&	21.4\%	&	85.1\%	\\	
    \multirow{2}{*}{Mistral-7B-Instruct}	&	Zero-Shot Classifier	&	21.0\%	&	52.7\%	&	47.1\%	\\	
    	&	Lora + Prompt	&	21.0\%	&	56.1\%	&	70.2\%	\\	
    \bottomrule
    \end{tabular}
    \vspace{1mm}
    \caption{
    ECE and AUROC on livecodebench\_generation\_lite (LeetCode easy subset).
    ECE is shown after temperature scaling on a small hold-out set of the original dataset mixture \cref{app:training-data}. Acc is task accuracy (proportion of coding solutions that are correct). Supervised training (LoRA + Prompt) seems to always improve selective prediction, although supervised training only heavily improves calibration for Mistral-7B and in fact slightly degrades calibration for the two other models.}
    \label{tab:coding}
\end{table}

\section{User Studies}
\label{app:user-study}

\subsection{Additional Details on Setup}

\paragraph{Stimuli and Participant Selection} We closely followed the setup of \citep{bhatt2023learning}. We used the same 180 MMLU questions from which were pre-batched into three sets of 60 MMLU questions. Within each variant, we randomly assigned participants to one of the three batches. In total, we recruit $181$ participants (20 per variant\footnote{With the exception of one extra participant due to random batching allocation effects.}). All participants were recruited through the crowdsourcing platform Prolific \citep{palan2018prolific}; we restrict our participant pool to those based in the United States who speak English as a first language.

\paragraph{Compensation} Participants were told that the study would take approximately 30 minutes and were paid at a base rate of \$9/hr and informed that they would receive an optional bonus up to \$10 for answering questions correctly. We applied the bonus to all participants. 

\paragraph{LLM Answers and Uncertainty Elicitation}
\citeauthor{bhatt2023learning} originally used GPT-3.5 as their LLM. While at first, we explored user performance when provided with confidence scores modulated over the original GPT-3.5 responses that the authors had collected, the authors had filtered LLM performance to ensure the LLM achieved high performance on biology, computer science, and foreign policy and poor performance on mathematics. As such, we noticed that participants overwhelmingly uptook the LLM's answer (which was rational behaviour, given the model's high performance). To explore a more nuanced performance profile, we regenerated LLM answers using Mistral 7B Instruct via greedy decoding. We then generated confidence scores on top of the LLM responses. For our random baseline, we sample a confidence score uniformly between 0 and 100\% for each question. 

\subsection{Important considerations}

There are many reasons to heed caution in interpreting our results as definitive indications of the utility of displaying confidence to users in LLM assistive settings. In particular: (i) users are presented with feedback after each trial as in \citep{bhatt2023learning} -- as such, they can determine (potentially rapidly) whether or not a model is reliable, even without confidence scores. However, in practical settings users may not know whether or not the model was truly correct and therefore confidence scores could have an even larger impact; (ii) MMLU questions can be challenging for non-experts -- we see the biggest differences in performance for the no-LLM vs. any-LLM-assistance condition. We may see a wider range of reliance behaviors in settings wherein people have more confidence in their own abilities; (iii) we present users with numeric confidence; however, humans are not always able to reliably process confidence estimates nor appropriately calibrate uncertainty estimates themselves~\citep{keren1991calibration, vodrahalli2022uncalibrated, collins2023human, lichtenstein1977calibration}. It may be that alternate modes of communicating confidence improve users' ability to appropriately leverage the confidence scores in their decision making process. We see targeted exploration of each component  through interdisciplinary collaboration across AI, behavioral science, and human-computer interaction as ripe for future work.

\subsection{Extended Results}

\paragraph{Task Accuracy and Reliance Sensibility}

We depict average user task accuracy and reliance sensibility across variants in Figure \ref{fig:user-study-extended}. We follow \citeauthor{bhatt2023learning} in computing reliance sensibility as the proportion of times the user appropriately sided with the model prediction when the model was correct and did not respond with the model's prediction when the model was incorrect. 

\begin{figure*}[!t]
    \centering
    \includegraphics[width=0.4\linewidth]{user_study_figs/agg_accs.pdf}
    \hspace{2mm}
    \includegraphics[width=0.4\linewidth]{user_study_figs/reliance_sensibility.pdf}
    \caption{
    (\textbf{Left}) User accuracy on 60 MMLU questions per variant ($N=20$ users per variant); violin plots show quartiles as dashed lines (\textbf{Right}) Average reliance sensibility (proportion of instances where the user sided with the model when the model was correct, and overrode the model's prediction when the model was incorrect); higher indicates better reliance calibration.}
    \label{fig:user-study-extended}
\end{figure*}

We depict per-topic accuracy, with the LLM's average performance in Figure \ref{fig:per-topic-acc-mistral}.

\begin{figure*}[!t]
    \centering
    \includegraphics[width=0.4\linewidth]{user_study_figs/high_school_biology_perf.pdf}
    \hspace{3mm}
    \includegraphics[width=0.4\linewidth]{user_study_figs/high_school_computer_science_perf.pdf} \\
    \vspace{3mm}
    \includegraphics[width=0.4\linewidth]{user_study_figs/us_foreign_policy_perf.pdf}
    \hspace{3mm}
    \includegraphics[width=0.4\linewidth]{user_study_figs/elementary_mathematics_perf.pdf}
    \caption{
    User accuracies per topic for the Mistral variants. Red line indicates the model's average accuracy.}
    \label{fig:per-topic-acc-mistral}
\end{figure*}

\paragraph{GPT-3.5 Confidence Generalization}

As noted, we ran variants using the same GPT-3.5 generations as \citep{bhatt2023learning}. We show aggregate and per-topic accuracy in \cref{fig:per-topic-acc-gpt35}, as well as reliance sensibility in \cref{fig:reliance-gpt35}. 

\begin{figure*}[!t]
    \centering
    \includegraphics[width=0.4\linewidth]{user_study_figs/high_school_biology_perf_gpt35.pdf}
    \hspace{3mm}
    \includegraphics[width=0.4\linewidth]{user_study_figs/high_school_computer_science_perf_gpt35.pdf} \\
    \vspace{3mm}
    \includegraphics[width=0.4\linewidth]{user_study_figs/us_foreign_policy_perf_gpt35.pdf}
    \hspace{3mm}
    \includegraphics[width=0.4\linewidth]{user_study_figs/elementary_mathematics_perf_gpt35.pdf}
    \caption{
    User accuracies per topic for the GPT-3.5 variants (with generalization confidence computed for the CT and Query cases). Red line indicates the model's average accuracy.}
    \label{fig:per-topic-acc-gpt35}
\end{figure*}

\begin{figure*}
    \centering
    \includegraphics[width=0.6\linewidth]{user_study_figs/reliance_sensibility_gpt35.pdf}
    \caption{
    Reliance sensibility for the variants based on GPT-3.5}
    \label{fig:reliance-gpt35}
\end{figure*}

\paragraph{Freeform User Responses}

We permitted users to provide freeform responses at the end of the study. Some users were sensitive to confidence scores being reported and came up with their own heuristics for whether to rely on the model's output. We include a sampling of comments across confidence variants: 

\begin{itemize}
 % mistral ct
    \item ``if it had a confidence of less than 50\% it made me very skeptical.'' 
    \item ``The model\'s confidence indeed helped me choose and select my answer as I trusted in them most of the time.''
    \item ``I didn\'t really rely on the confidence level. If I had 0 confidence in the answer myself I relied on the AI regardless.''
    % gpt-3.5 ct
    \item ``if the models confidence fell below 45 I decided to investigate it myself by remembering pieces of information. and also reasoning the question. If it was above 45 I would automatically agree to its prediction but there were some few cases I  challenged it even though it was above 45''
    \item ``At first I was hesistant to trust the model much because of the lower confidence levels but I still trusted it enough on topics I struggled with. As it went on, I was comfortable with confidence levels above 40.''
    \item ``If the model\'s confidence was low and I thought I knew the answer (and it was different) I chose my answer''
\end{itemize}

\subsection{Interface and Instructions}
\label{app:user-study-interfact}

We show a sample interface of our extension of \texttt{Modiste} with user confidence in Figure \ref{fig:modiste-confidence}, and present the the full set of instructions provided to users in Figures \ref{fig:experiment-instructions} and \ref{fig:experiment-instructions-2}. Note, for the LLM-only and no-LLM conditions, we followed the instruction text from \citep{bhatt2023learning} directly, i.e., participants who saw only the LLM did not see the instruction page about model confidence, and participants in the ``No-LLM'' variant were not instructed about any model variant and were just instructed to answer the questions as best as they could by themselves. Participants also responded to a post survey questionarre after completing the user study, which we depict in Figure \ref{fig:postquestionarre}.

\begin{figure}
    \centering
    \includegraphics[width=0.7\linewidth]{user_study_figs/instructions/page_with_feedback.png}
    \caption{Example interface from \texttt{Modiste}. Participants are informed of the question (and topic), as well as the LLM prediction and confidence. Participants are informed of their running score throughout the experiment.}
    \label{fig:modiste-confidence}
\end{figure}

\begin{figure}
    \centering
    \includegraphics[width=0.8\linewidth]{user_study_figs/instructions/starter_inst.png}
    \includegraphics[width=0.8\linewidth]{user_study_figs/instructions/likely_answer_inst.png}
    \includegraphics[width=0.8\linewidth]{user_study_figs/instructions/ai_pred_inst.png}
    \includegraphics[width=0.8\linewidth]{user_study_figs/instructions/confidence_inst.png}
    \includegraphics[width=0.8\linewidth]{user_study_figs/instructions/seconds_per.png}
    \includegraphics[width=0.8\linewidth]{user_study_figs/instructions/bonus.png}
    \caption{Experiment instructions for the confidence variants.}
    \label{fig:experiment-instructions}
\end{figure}

\begin{figure}
    \centering
    
    \includegraphics[width=0.8\linewidth]{user_study_figs/instructions/questions.png}
    \includegraphics[width=0.8\linewidth]{user_study_figs/instructions/next.png}
    \includegraphics[width=0.8\linewidth]{user_study_figs/instructions/mc_check.png}
    \caption{Experiment instructions for the confidence variants (continued).}
    \label{fig:experiment-instructions-2}
\end{figure}

\begin{figure}
    \centering
    \includegraphics[width=0.9\linewidth]{user_study_figs/instructions/postsurvey_questionarre.png}
    \caption{Sample pot-survey questionnaire for users who were allocated to a variant wherein they saw model confidence.}
    \label{fig:postquestionarre}
\end{figure}

\section{Broader Impact and Implications}
\label{app:broader-impact}

The goal of this work is to make LLM outputs have better confidence values associated with them. 
With successful, calibrated confidence values, the machine systems ultimately become more interpretable and trustworthy by a user~\citep{janssen2008updating}. 
When applied correctly, our advancements will help users be able to make decisions based off of LLM outputs in a more informed way.
Similar examples in other domains, like AlphaFold~\cite{terwilliger2023alphafold}, have shown how well-calibrated confidence scores can be useful in complex decision-making domains.
Our hope is to replicate those broad findings in LLMs.

We acknowledge the ongoing debate over the appropriateness, limitations, and harms of LLMs. 
We do highlight that the development of more confident, interpretable, and trustworthy LLMs can lead to continued techno-solutionism in unintended applications. 
Specifically, we highlight that our work is limited to use-cases with fact-based questions.
Many applications of text-based LLMs are generative, meaning that there is no way for our paradigm to be applied appropriately, and the use of a confidences from calibration-tuned models could be misleading or damaging without checks and guardrails.
Additionally, even within the fact-based paradigm, what is true can be subjective, with ground truth in machine learning being a contested topic~\citep{aroyo2015truth, uma2021learning}.

The philosophical debate on these topics is beyond the expertise of the authors; nonetheless, we believe that the ongoing debate over the appropriateness of LLMs should be considered in context with the benefits of our approach in making LLMs more interpretable and useful.
